# Supplementary material for: A Paragraph-level Multi-task Learning Model for Scientific Fact-Verification
Source: arXiv:2012.14500 source file (2021-01-25)
Supplement: Supplementary file 1 [file aaai2021_appendix.tex]

\appendix

\section{Appendices}
\label{sec:appendix}
